# Supplementary material for: Estimating the Contamination Factor's Distribution in Unsupervised Anomaly Detection
Source: arXiv:2210.10487 source file (2023-10-17)
Supplement: Supplementary file 1 [file supplement.tex]

%\documentclass[twoside]{article}

%\usepackage{aistats2023}
%\input{packages}
% If your paper is accepted, change the options for the package
\newpage
\appendix
\onecolumn
\section*{Supplementary Materials}

This Supplement contains additional details about our method and the experiments.

\section{Methodology}
In this section, we further explain (1) how to find the optimal values of our hyperparameters $\delta$ and $\tau$, and (2) how to collect samples from our estimate of $\gamma|S$ posterior. Moreover, we provide (3) additional technical details to reproduce the code.

\paragraph{1. Finding the values of $\delta$ and $\tau$.}  \lorenzo{IT'S IN THE PAPER}
We introduce two new hyperparameters $\delta$ and $\tau$ that have the role of properly calibrating the sigmoid function. By setting the following equations:
\begin{align*}
    p_0 &= 1 - \Pp (c_1) = 1 - \frac{1}{1+ e^{(\tau + \delta \cdot r(\tilde{\mu}_1, \tilde{\Sigma}_1))}}\\
    p_{\rm high} &= \Pp (\gamma \ge t|S ) = \sum_{k = 1}^K \changed{\Pp(C^* = k)} \cdot \Pp \left(\sum_{j = 1}^k \pi_j\ge t|S \right)
\end{align*}
we aim at finding the unique (optimal) value of $\delta$ and $\tau$. We solve the optimization problem using the least square optimizer as implemented in \textsc{SkLearn}.\footnote{\url{https://docs.scipy.org/doc/scipy/reference/generated/scipy.optimize.least_squares.html}}

However, while we can always find some values such that the first condition holds (on $p_0$), the second one can be satisfied only if $p_{\rm high} \ge \Pp(\pi_1 \ge t)$. Experimentally $\pi_1$ has almost always low values, which means $\Pp(\pi_1 \ge t) = 0$ for $t=0.15$. However, in case the such a constraint cannot be satisfied, we keep running again the variational inference method (with different starting point) for the DPGMM until the constraint on $p_{\rm high}$ holds. If this cannot happen or does not happen within $100$ iterations, we reject the possibility of too high contamination factors and just set it to $0$. 

\paragraph{2. Sampling algorithm.} \lorenzo{IT'S IN THE PAPER}
After creating the $M$-dimensional space using the $M$ anomaly detectors, we fit the DPGMM model and obtain an approximation for the posterior $p(\pi, \mu, \Sigma | S)$.
Then we derive a sample from $p(\gamma|S)$ in four steps by repeating the next operations for all $k \le K$.
First, we draw a sample $\pi_k^{(z)}, \mu_k^{(z)}, \Sigma_k^{(z)}$ from $\pi_k$ (Dirichlet), $\mu_k$ (Normal), $\Sigma_k$ (Inverse Wishart). 
Second, we transform $\pi_k^{(z)}$ by taking the cumulative sum and obtain a sample $\sum_{j = 1}^k \pi_j^{(z)}$. 
Third, we pass $\mu_k^{(z)}$ and $\Sigma_k^{(z)}$ through the sigmoid function (Eq.2) to get the conditional probabilities $\Pp(c_k \ | \ c_{k-1})$, and transform them into the exact joint probabilities $\Pp(C^* = k)$ using the equation 3. 
Finally, we multiply the samples following Formula 4 and obtain a sample $\gamma^{(z)}$ from $p(\gamma|S)$.

\paragraph{3. Additional technical details.}  \lorenzo{IT'S IN THE PAPER}
Because our method uses the variational inference approximation, we run it $10$ times and concatenate the samples to reduce the risk of biased distributions due to local minima. Moreover, after sorting the components, we set $\Pp(c_{k} | c_{k-1}) = 0$ for all $k > K' = \argmax \{k \colon \  \E[\sum_{j=1}^k \pi_j] < 0.25 \}$. This has the effect of setting an upper bound of $0.25$ to the contamination factor $\gamma$.
Because anomalies must be rare, we realistically assume that it is not possible to have more than $25\%$ of them. \changed{Although ``$0.25$'' could be considered a hyperparameter, this value has virtually no impact on the experimental results.} Moreover, note that $\E[\pi_1] \ge 0.25$ cannot occur, as otherwise we could not set the hyperparameters $p_0$ and $p_{\rm high}$.

\section{Experiments}
In this section we explain the threshold estimators and the ten anomaly detectors used by \ourmethod{} to assign the anomaly scores. Moreover, we provide additional details on the datasets used, and we extend the results of Q1,Q2 and Q3.

\paragraph{Threshold estimators.}\lorenzo{IT'S IN THE PAPER}
In statistics there are several methods that, given mono-dimensional scores belonging to two distributions, set a threshold to split them. These methods can be applied in our setting to estimate the contamination factor as the proportion of examples greater than the set threshold.
We cluster these statistical methods in $9$ groups:
\newline
\emph{1. Kernel-based.}
\textsc{Fgd}~\citep{qi2021iterative} and \textsc{Aucp}~\citep{ren2018robust} both use the kernel density estimator to estimate the score density; \textsc{Fgd} exploits the inflection points of the density's first derivative, while \textsc{Aucp} uses the percentage of the total kernel density estimator's AUC to set the threshold;
\newline
\emph{2. Curve-based.}
\textsc{Eb}~\citep{friendly2013elliptical} creates elliptical boundaries by generating pseudo-random eccentricities, while \textsc{Wind}~\citep{jacobson2013robust} is based on the topological winding number with respect to the origin;
\newline
\emph{3. Normality-based.}
\textsc{Zscore}~\citep{bagdonavivcius2020multiple} exploits the Z-scores, \textsc{Dsn}~\citep{amagata2021fast} measures the distance shift from a normal distribution, and \textsc{Chau}~\citep{bol1975chauvenet} follows the Chauvenet’s criterion before using the Z-score;
\newline
\emph{4. Regression-based.}
\textsc{Clf} and \textsc{Regr}~\citep{aggarwal2017introduction} are two regression models that separate the anomalies based on the y-intercept value;
\newline
\emph{5. Filter-based.}
\textsc{Filter}~\citep{hashemi2019filtering}, and \textsc{Hist}~\citep{thanammal2014effective} use, respectively, the wiener filter and the Otsu's method to filter out the anomalous scores;
\newline
\emph{6. Statistical test-based.}
\textsc{Gesd}~\citep{alrawashdeh2021adjusted}, \textsc{Mcst}~\citep{coin2008testing} and \textsc{Mtt}~\citep{rengasamy2021towards} are based on, respectively, the generalized extreme studentized, the Shapiro-Wilk, and the modified Thompson Tau statistical tests;
\newline
\emph{7. Statistical moment-based.}
\textsc{Boot}~\citep{martin2006evaluation} derives the confidence interval through the two sided bias-corrected and accelerated bootstrap; \textsc{Karch}~\citep{afsari2011riemannian} and \textsc{Mad}~\citep{archana2015periodicity} are based on means and standard deviations, i.e., respectively, the Karcher mean plus one standard deviation, and the mean plus the median absolute deviation over the standard deviation;
\newline
\emph{8. Quantile-based.}
\textsc{Iqr}~\citep{bardet2017new} and \textsc{Qmcd}~\citep{iouchtchenko2019deterministic} set the threshold based on quantiles, i.e., respectively, the third quartile $Q_3$ plus $1.5$ times the inter-quartile region $|Q_3 - Q_1|$, and the quantile of one minus the Quasi-Monte Carlo discreprancy;
\newline
\emph{9. Transformation-based.}
\textsc{Moll}~\citep{keyzer1997using} smooths the scores through the Friedrichs’ mollifier, while \textsc{Yj}~\citep{raymaekers2021transforming} applies the Yeo-Johnson monotonic transformations.

\paragraph{Anomaly Detectors.} \lorenzo{IT'S IN THE PAPER}
We use $10$ anomaly detectors with different inductive biases: \textsc{kNN}~\citep{angiulli2002fast}
assumes that the anomalies are far away from normals, \textsc{IForest}~\citep{liu2012isolation} assumes that the anomalies are easier to isolate, \textsc{LOF}~\citep{breunig2000lof} exploits the examples' density, \textsc{OCSVM}~\citep{green2001modelling} encapsulates the data into a multi-dimensional hypersphere, \textsc{Ae}~\citep{chen2018autoencoder} and \textsc{VAE}~\citep{kingma2013auto} use the reconstruction error as anomaly score function in a, respectively, deterministic and probabilistic perspective, \textsc{LSCP}~\citep{zhao2019lscp} is an ensemble method that selects competent detectors locally, \textsc{HBOS}~\citep{goldstein2012histogram} calculates the degree of anomalousness by building histograms, \textsc{LODA}~\citep{pevny2016loda} is an ensemble of weak detectors that build histograms on randomly generated projected spaces, and \textsc{COPOD}~\citep{li2020copod} is a copula based method. All these methods are implemented in the python library PyOD~\citep{zhao2019pyod}.

\paragraph{Data.}
\begin{table}[]
\caption{Properties of the $22$ datasets used. For each dataset, we report the number examples, the number of original covariates, and the ground-truth contamination factor.}
\label{tab:data}
\centering
\begin{tabular}{lrrr}
\toprule
Dataset & \# Examples (N) & \# Covariates & True $\gamma^*$\\
\midrule
ALOI             &12384      &27          &0.0304 \\
Annthyroid       &7129       &21          &0.0749 \\
Arrhythmia       &271        &259         &0.0996 \\
Cardiotocography &1734       &21          &0.0496 \\
Glass            &214        &7           &0.0421 \\
InternetAds      &1682       &1555        &0.0499 \\
KDDCup99         &48113      &40          &0.0042 \\
Lymphography     &148        &47          &0.0405 \\
PageBlocks       &5473       &10          &0.1023 \\
Parkinson        &53         &22          &0.0943 \\
PenDigits        &9868       &16          &0.0020 \\
Pima             &526        &8           &0.0494 \\
Shuttle          &1013       &9           &0.0128 \\
SpamBase         &2661       &57          &0.0500 \\
Stamps           &340        &9           &0.0912 \\
T15              &42125      &10          &0.0668 \\
T21              &18509      &10          &0.0529 \\
WBC              &223        &9           &0.0448 \\
WDBC             &367        &30          &0.0272 \\
WPBC             &160        &33          &0.0562 \\
Waveform         &3443       &21          &0.0290 \\
Wilt             &4655       &5           &0.0200 \\
\bottomrule
\end{tabular}
\end{table}

Table~\ref{tab:data} shows the details of the used datasets. The datasets vary in terms of number of examples (from around $50$ to more than $48000$), number of covariates (from $5$ to more than $1500$) and the contamination factor (from around $0.004$ to more than $0.10$). Note that even the highest contamination factor is around $0.10$, confirming the general assumption of anomalies being rare.

\paragraph{Q1-Q2. \ourmethod{}'s estimated distribution.}

\begin{figure*}[h]
\vspace{.1in}
\centerline{\includegraphics[width=.99\textwidth]{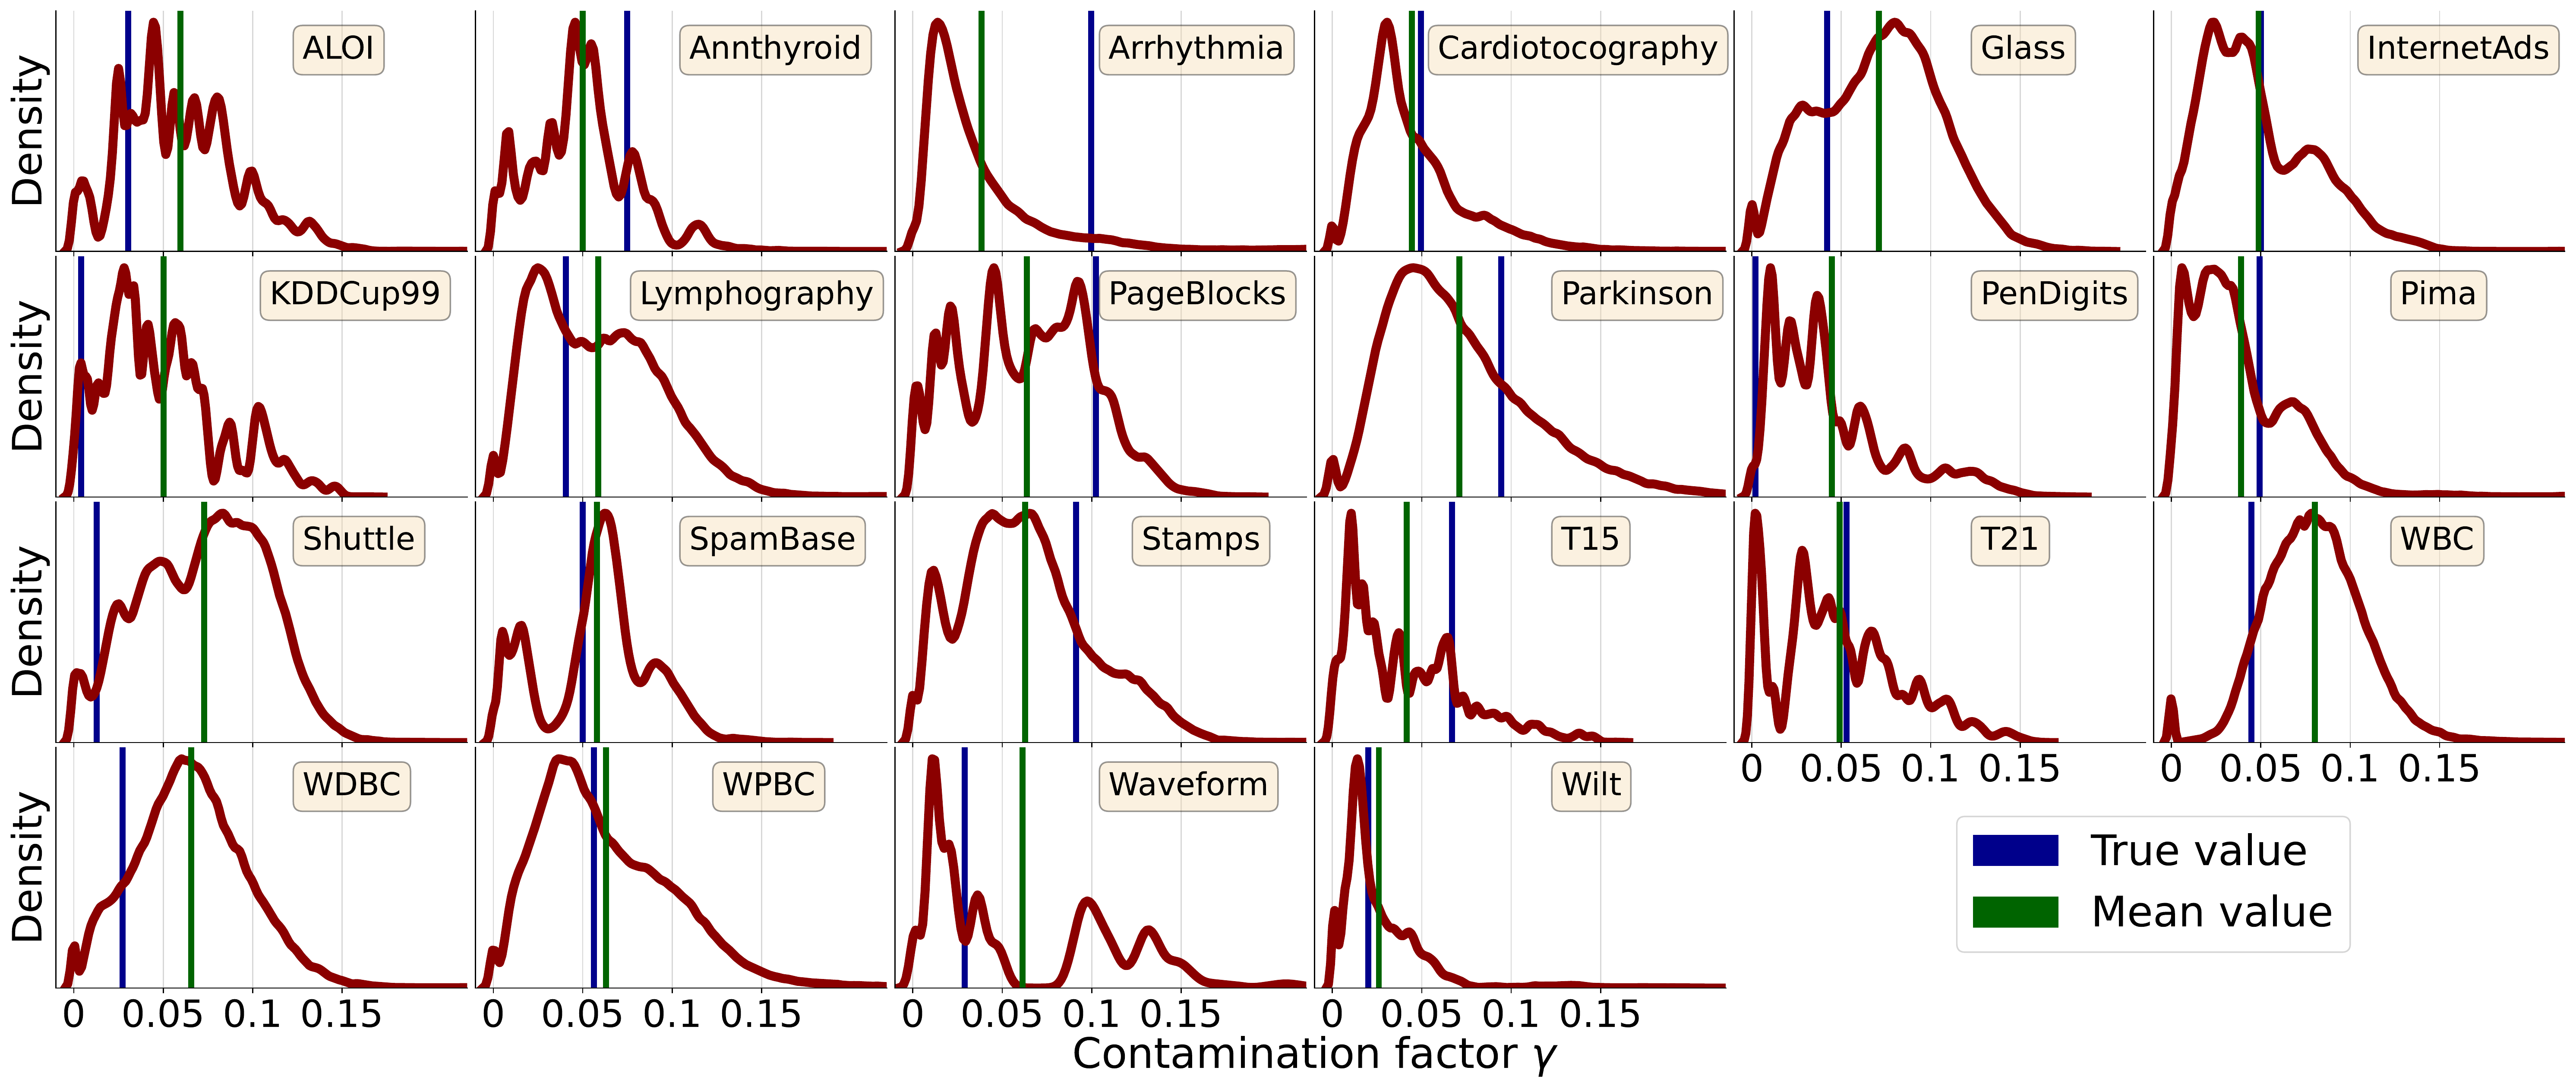}}
\vspace{.1in}
\caption{Illustration of how \ourmethod{} estimates $\gamma$'s posterior on the $22$ datasets. }\label{fig:22densities}
\end{figure*}

\begin{table}[h]
\centering
\caption{Mean Absolute Error (MAE) between the true contamination factor and \ourmethod{}'s sample mean for the $22$ datasets.}
\label{tab:MAE_values}
\begin{tabular}{lccc}
\toprule
Dataset & \ourmethod{}'s sample mean & True $\gamma^*$ &     MAE \\
\midrule
ALOI             &      0.0596 &          0.0304 &  0.0292 \\
Annthyroid       &      0.0499 &          0.0749 &  0.0250 \\
Arrhythmia       &      0.0385 &          0.0996 &  0.0611 \\
Cardiotocography &      0.0446 &          0.0496 &  0.0050 \\
Glass            &      0.0711 &          0.0421 &  0.0290 \\
InternetAds      &      0.0487 &          0.0499 &  0.0012 \\
KDDCup99         &      0.0502 &          0.0042 &  0.0460 \\
Lymphography     &      0.0587 &          0.0405 &  0.0182 \\
PageBlocks       &      0.0638 &          0.1023 &  0.0385 \\
Parkinson        &      0.0711 &          0.0943 &  0.0232 \\
PenDigits        &      0.0446 &          0.0020 &  0.0426 \\
Pima             &      0.0390 &          0.0494 &  0.0104 \\
Shuttle          &      0.0728 &          0.0128 &  0.0600 \\
SpamBase         &      0.0580 &          0.0500 &  0.0080 \\
Stamps           &      0.0627 &          0.0912 &  0.0285 \\
T15              &      0.0417 &          0.0668 &  0.0251 \\
T21              &      0.0490 &          0.0529 &  0.0039 \\
WBC              &      0.0802 &          0.0448 &  0.0354 \\
WDBC             &      0.0657 &          0.0272 &  0.0385 \\
WPBC             &      0.0631 &          0.0562 &  0.0069 \\
Waveform         &      0.0614 &          0.0290 &  0.0324 \\
Wilt             &      0.0260 &          0.0200 &  0.0060 \\
\bottomrule
\end{tabular}
\end{table}

Figure~\ref{fig:22densities} shows our estimate of $\gamma|S$'s posterior on the $22$ used datasets. Moreover, Table~\ref{tab:MAE_values} shows the MAE between \ourmethod{}'s sample mean and the true value $\gamma^*$ on a per-dataset basis.
With respect to the true value $\gamma^*$ and out of $22$ experiments, the sample mean is: 
\begin{itemize}
    \item a \emph{good estimate} (i.e., MAE $\le 0.01$) for $7$ datasets (Cardiotocography, InternetAds, Pima, SpamBase, T21, WPBC, Wilt);
    \item a \emph{slightly imprecise estimate} (i.e., $0.01 < $ MAE $\le 0.03$) for $7$ datasets (ALOI, Annthyroid, Glass, Lymphography, Parkinson, Stamps and T15);
    \item a \emph{not-optimal estimate} (i.e., $0.03 < $ MAE $\le 0.05$) for $6$ datasets (KDDCup99, PageBlocks, PenDigits, WBC, WDBC, and Waveform);
    \item a \emph{bad estimate} (MAE $> 0.05$) for just two datasets (Arrhythmia, and Shuttle).
\end{itemize}   
This shows, again, that the estimated distribution is well-calibrated.

\paragraph{Q3. Selecting the anomaly detectors to compute the $F_1$ score.}
\begin{table}[h]
\caption{List of detectors with the greatest $F_1$ score when using the true contamination factor to set the threshold. For each dataset, we use such subset of detectors to compute the deterioration.} \label{tab:detectorsperexperiment}
\begin{center}
\begin{tabular}{lll}
\toprule
        Dataset &                           Anomaly Detectors \\
\midrule
      ALOI &                                                KNN \\
Annthyroid &                                               HBOS \\
Arrhythmia &                                 IForest-HBOS-COPOD \\
Cardiotocography &                                        KNN \\
     Glass &                                                LOF \\
  InternetAds &                                               LSCP \\
  KDDCup99 &                                              COPOD \\
 Lymphography &                                 KNN-LOF-OCSVM-HBOS \\
PageBlocks &                                                LOF \\
 Parkinson &                    LSCP-HBOS-COPOD-LSCP-HBOS-COPOD \\
 PenDigits &  KNN-IForest-LOF-OCSVM-LSCP-Ae-VAE-HBOS-LODA-COPOD \\
      Pima &                                            IForest \\
   Shuttle &        KNN-OCSVM-Ae-VAE-HBOS-KNN-OCSVM-Ae-VAE-HBOS \\
  SpamBase &                                               LSCP \\
    Stamps &                                               LSCP \\
       T15 &                                              OCSVM \\
       T21 &                                              OCSVM \\
       WBC &                           KNN-LOF-OCSVM-LODA-COPOD \\
      WDBC &               KNN-LOF-OCSVM-LSCP-Ae-VAE-LODA-COPOD \\
      WPBC &                                              OCSVM \\
  Waveform &                                              OCSVM \\
      Wilt &                                                LOF \\
\bottomrule
\end{tabular}

\end{center}
\end{table}

Because we aim at studying the effect of the contamination factor on the detectors' performance, we compare the $F_1$ scores only over the detectors that work well for each of the dataset. 
For each dataset $D$, we use as set of detectors those achieving the greatest $F_1$ score using the true contamination factor, i.e. $\argmax_{f_m} \left\{F_1 (f_m, D, \gamma^*)\right\}$. This means that, for each dataset, we (1) use each detector separately to make predictions using the true contamination factor $\gamma^*$, (2) measure their $F_1$ score, (3) keep those detectors that obtains the greatest $F_1$, and (4) use them to compute the $F_1$ deterioration using the point-estimates of the contamination factor. Table~\ref{tab:detectorsperexperiment} lists the detectors used for each dataset to compute the $F_1$ deterioration. Observe that sometimes only a single detector obtains the greatest $F_1$ score, while sometimes several detectors get the same $F_1$ score.

\paragraph{Q3. False alarms and false negatives.}

\begin{table}[h]
\caption{Mean and standard deviation of the false alarm rate (left) and false negative rate (right) obtained by using each method's $\gamma$ estimate to set the threshold (the lower the better). Regarding the false alarms, \ourmethod{} has the third best mean and outperforms \textsc{Qmcd} and \textsc{Karch}, which are the second and third best baseline when measuring the $F_1$ score. On the other hand, \ourmethod{} obtains higher false negative rates than almost all the competitors, due to the fact that the threshold estimators overestimate the true contamination factor.} \label{tab:false_alarms}
\begin{center}
\begin{tabular}{lc}
\multicolumn{2}{c}{\textbf{False Alarm Rate}} \\
\toprule
Method &      Mean $\pm$ std. \\
\midrule
\textsc{Iqr}                 &  $0.009 \pm 0.008$               \\
\textsc{Mtt}                 &  $0.027 \pm  0.024$              \\
\textbf{$\gamma$\textsc{GMM}}&\textbf{0.042}$\pm$\textbf{0.015} \\
\textsc{Qmcd}                &  $0.059 \pm  0.018$              \\
\textsc{Karch}               &  $0.147 \pm  0.047$              \\
\textsc{Chau}                &  $0.190 \pm  0.035$              \\
\textsc{Zscore}              &  $0.221 \pm  0.050$               \\
\textsc{Yj}                  &  $0.390 \pm  0.139$            \\
\textsc{Filter}              &  $0.454 \pm  0.054$        \\
\textsc{Dsn}                 &  $0.477 \pm  0.134$          \\
\textsc{Hist}                &  $0.513 \pm  0.100$         \\
\textsc{Fgd}                 &  $0.533 \pm  0.183$      \\
\textsc{Aucp}                &  $0.591 \pm  0.088$      \\
\textsc{Mcst}                &  $0.611 \pm  0.287$       \\
\textsc{Gesd}                &  $0.616 \pm  0.106$      \\
\textsc{Regr}                &  $0.643 \pm  0.105$      \\
\textsc{Mad}                 &  $0.731 \pm  0.083$       \\
\textsc{Clf}                 &  $0.757 \pm  0.077$      \\
\textsc{Eb}                  &  $0.785 \pm  0.077$       \\
\textsc{Wind}                &  $0.809 \pm  0.076$      \\
 \textsc{Moll}               &  $0.816 \pm  0.082$      \\
 \textsc{Boot}               &  $0.862 \pm  0.079$      \\

\bottomrule
\end{tabular}
\qquad
\begin{tabular}{lc}
\multicolumn{2}{c}{\textbf{False Negative Rate}} \\
\toprule
Method &      Mean $\pm$ std \\
\midrule
 \textsc{Boot} &  $0.001 \pm  0.002$ \\
 \textsc{Wind} &  $0.001 \pm  0.002$ \\
 \textsc{Moll} &  $0.001 \pm  0.002$ \\
   \textsc{Eb} &  $0.001 \pm  0.003$ \\
  \textsc{Mad} &  $0.002 \pm  0.003$ \\
  \textsc{Clf} &  $0.002 \pm  0.003$ \\
 \textsc{Gesd} &  $0.003 \pm  0.005$ \\
 \textsc{Regr} &  $0.003 \pm  0.005$ \\
 \textsc{Aucp} &  $0.004 \pm  0.006$ \\
 \textsc{Hist} &  $0.006 \pm  0.008$ \\
  \textsc{Fgd} &  $0.007 \pm  0.011$ \\
  \textsc{Dsn} &  $0.007 \pm  0.009$ \\
  \textsc{Filter} &  $0.007 \pm  0.009$ \\
 \textsc{Mcst} &  $0.007 \pm  0.012$ \\
   \textsc{Yj} &  $0.009 \pm  0.010$ \\
  \textsc{Zscore} &  $0.017 \pm  0.015$ \\
 \textsc{Chau} &  $0.019 \pm  0.016$ \\
\textsc{Karch} &  $0.021 \pm  0.018$ \\
 \textsc{Qmcd} &  $0.034 \pm  0.024$ \\
\bf{$\gamma$GMM} &  \bf{0.036 $\pm$  0.025} \\
  \textsc{Mtt} &  $0.042 \pm  0.028$ \\
  \textsc{Iqr} &  $0.044 \pm  0.029$ \\
\bottomrule
\end{tabular}

\end{center}
\end{table}

Finally, Table~\ref{tab:false_alarms} shows the false alarm (false positive) rate and the false negative rate. The majority of the threshold estimators provide extremely high estimates for the contamination factor, shown here as extremely low false negative rates, but they would be useless in practice because of their high false alarm rate. In fact, this metric is important as false alarms result in real costs for the company (e.g., turning the wind turbine off to wait until the ice on the blades melts down), while reducing trust in the detection system. Our method reduces the false alarm rate compared to most of the baselines, including \textsc{Qmcd} and \textsc{Karch} that achieve the second and third best $F_1$ scores on average. On the other hand, \textsc{Iqr} and \textsc{Mtt} have the lowest false positive rates, due to the fact that they often underestimate the contamination factor as supported by the false negative table.

%\section{FORMATTING INSTRUCTIONS}

%To prepare a supplementary pdf file, we ask the authors to use \texttt{aistats2022.sty} as a style file and to follow the same formatting instructions as in the main paper.
%The only difference is that the supplementary material must be in a \emph{single-column} format.
%You can use \texttt{supplement.tex} in our starter pack as a starting point, or append the supplementary content to the main paper and split the final PDF into two separate files.

%Note that reviewers are under no obligation to examine your supplementary material.

%\section{MISSING PROOFS}

%The supplementary materials may contain detailed proofs of the results that are missing in the main paper.

%\subsection{Proof of Lemma 3}

%\textit{In this section, we present the detailed proof of Lemma 3 and then [ ... ]}

%\section{ADDITIONAL EXPERIMENTS}

%If you have additional experimental results, you may include them in the supplementary materials.

%\subsection{The Effect of Regularization Parameter}

%\textit{Our algorithm depends on the regularization parameter $\lambda$. Figure 1 below illustrates the effect of this parameter on the performance of our algorithm. As we can see, [ ... ]}

%\bibliography{bibliography}

%\end{document}
