# Supplementary material for: Estimating the Contamination Factor's Distribution in Unsupervised Anomaly Detection
Source: arXiv:2210.10487 source file (2023-10-17)
Supplement: Supplementary file 2 [file OnlineSupplement.tex]

\newpage
\appendix
\onecolumn
\section*{Supplementary Materials}

This online Supplement contains additional details about the experiments. Specifically, we provide additional details on the datasets used, and we extend the results of Q1,Q2 and Q3.

\paragraph{Data.}
\begin{table}[htbp]
\caption{Properties of the $22$ datasets used. For each dataset, we report the number examples, the number of original covariates, and the ground-truth contamination factor.}
\label{tab:data}
\centering
\begin{tabular}{lrrr}
\toprule
Dataset & \# Examples (N) & \# Covariates & True $\gamma^*$\\
\midrule
ALOI             &12384      &27          &0.0304 \\
Annthyroid       &7129       &21          &0.0749 \\
Arrhythmia       &271        &259         &0.0996 \\
Cardiotocography &1734       &21          &0.0496 \\
Glass            &214        &7           &0.0421 \\
InternetAds      &1682       &1555        &0.0499 \\
KDDCup99         &48113      &40          &0.0042 \\
Lymphography     &148        &47          &0.0405 \\
PageBlocks       &5473       &10          &0.1023 \\
Parkinson        &53         &22          &0.0943 \\
PenDigits        &9868       &16          &0.0020 \\
Pima             &526        &8           &0.0494 \\
Shuttle          &1013       &9           &0.0128 \\
SpamBase         &2661       &57          &0.0500 \\
Stamps           &340        &9           &0.0912 \\
T15              &42125      &10          &0.0668 \\
T21              &18509      &10          &0.0529 \\
WBC              &223        &9           &0.0448 \\
WDBC             &367        &30          &0.0272 \\
WPBC             &160        &33          &0.0562 \\
Waveform         &3443       &21          &0.0290 \\
Wilt             &4655       &5           &0.0200 \\
\bottomrule
\end{tabular}
\end{table}

Table~\ref{tab:data} shows the details of the used datasets. The datasets vary in terms of number of examples (from around $50$ to more than $48000$), number of covariates (from $5$ to more than $1500$) and the contamination factor (from around $0.004$ to more than $0.10$). Note that even the highest contamination factor is around $0.10$, confirming the general assumption of anomalies being rare.

\paragraph{Q1-Q2. \ourmethod{}'s estimated distribution.}

\begin{table}[htpb]
\centering
\caption{Mean Absolute Error (MAE) between the true contamination factor and \ourmethod{}'s sample mean for the $22$ datasets.}
\label{tab:MAE_values}
\begin{tabular}{lccc}
\toprule
Dataset & \ourmethod{}'s sample mean & True $\gamma^*$ &     MAE \\
\midrule
ALOI             &      0.0596 &          0.0304 &  0.0292 \\
Annthyroid       &      0.0499 &          0.0749 &  0.0250 \\
Arrhythmia       &      0.0385 &          0.0996 &  0.0611 \\
Cardiotocography &      0.0446 &          0.0496 &  0.0050 \\
Glass            &      0.0711 &          0.0421 &  0.0290 \\
InternetAds      &      0.0487 &          0.0499 &  0.0012 \\
KDDCup99         &      0.0502 &          0.0042 &  0.0460 \\
Lymphography     &      0.0587 &          0.0405 &  0.0182 \\
PageBlocks       &      0.0638 &          0.1023 &  0.0385 \\
Parkinson        &      0.0711 &          0.0943 &  0.0232 \\
PenDigits        &      0.0446 &          0.0020 &  0.0426 \\
Pima             &      0.0390 &          0.0494 &  0.0104 \\
Shuttle          &      0.0728 &          0.0128 &  0.0600 \\
SpamBase         &      0.0580 &          0.0500 &  0.0080 \\
Stamps           &      0.0627 &          0.0912 &  0.0285 \\
T15              &      0.0417 &          0.0668 &  0.0251 \\
T21              &      0.0490 &          0.0529 &  0.0039 \\
WBC              &      0.0802 &          0.0448 &  0.0354 \\
WDBC             &      0.0657 &          0.0272 &  0.0385 \\
WPBC             &      0.0631 &          0.0562 &  0.0069 \\
Waveform         &      0.0614 &          0.0290 &  0.0324 \\
Wilt             &      0.0260 &          0.0200 &  0.0060 \\
\bottomrule
\end{tabular}
\end{table}

Table~\ref{tab:MAE_values} shows the MAE between \ourmethod{}'s sample mean and the true value $\gamma^*$ on a per-dataset basis.
With respect to the true value $\gamma^*$ and out of $22$ experiments, the sample mean is: 
\begin{itemize}
    \item a \emph{good estimate} (i.e., MAE $\le 0.01$) for $7$ datasets (Cardiotocography, InternetAds, Pima, SpamBase, T21, WPBC, Wilt);
    \item a \emph{slightly imprecise estimate} (i.e., $0.01 < $ MAE $\le 0.03$) for $7$ datasets (ALOI, Annthyroid, Glass, Lymphography, Parkinson, Stamps and T15);
    \item a \emph{not-optimal estimate} (i.e., $0.03 < $ MAE $\le 0.05$) for $6$ datasets (KDDCup99, PageBlocks, PenDigits, WBC, WDBC, and Waveform);
    \item a \emph{bad estimate} (MAE $> 0.05$) for just two datasets (Arrhythmia, and Shuttle).
\end{itemize}   
This shows, again, that the estimated distribution is well-calibrated.

\paragraph{Q3. Selecting the anomaly detectors to compute the $F_1$ score.}
\begin{table}[h]
\caption{List of detectors with the greatest $F_1$ score when using the true contamination factor to set the threshold. For each dataset, we use such a subset of detectors to compute the deterioration.} \label{tab:detectorsperexperiment}
\begin{center}
\begin{tabular}{lll}
\toprule
        Dataset &                           Anomaly Detectors \\
\midrule
      ALOI &                                                KNN \\
Annthyroid &                                               HBOS \\
Arrhythmia &                                 IForest-HBOS-COPOD \\
Cardiotocography &                                        KNN \\
     Glass &                                                LOF \\
  InternetAds &                                               LSCP \\
  KDDCup99 &                                              COPOD \\
 Lymphography &                                 KNN-LOF-OCSVM-HBOS \\
PageBlocks &                                                LOF \\
 Parkinson &                    LSCP-HBOS-COPOD-LSCP-HBOS-COPOD \\
 PenDigits &  KNN-IForest-LOF-OCSVM-LSCP-Ae-VAE-HBOS-LODA-COPOD \\
      Pima &                                            IForest \\
   Shuttle &        KNN-OCSVM-Ae-VAE-HBOS-KNN-OCSVM-Ae-VAE-HBOS \\
  SpamBase &                                               LSCP \\
    Stamps &                                               LSCP \\
       T15 &                                              OCSVM \\
       T21 &                                              OCSVM \\
       WBC &                           KNN-LOF-OCSVM-LODA-COPOD \\
      WDBC &               KNN-LOF-OCSVM-LSCP-Ae-VAE-LODA-COPOD \\
      WPBC &                                              OCSVM \\
  Waveform &                                              OCSVM \\
      Wilt &                                                LOF \\
\bottomrule
\end{tabular}

\end{center}
\end{table}

Because we aim at studying the effect of the contamination factor on the detectors' performance, we compare the $F_1$ scores only over the detectors that work well for each of the datasets. 
For each dataset $D$, we use as set of detectors those achieving the greatest $F_1$ score using the true contamination factor, i.e. $\argmax_{f_m} \left\{F_1 (f_m, D, \gamma^*)\right\}$. This means that, for each dataset, we (1) use each detector separately to make predictions using the true contamination factor $\gamma^*$, (2) measure their $F_1$ score, (3) keep those detectors that obtain the greatest $F_1$, and (4) use them to compute the $F_1$ deterioration using the point-estimates of the contamination factor. Table~\ref{tab:detectorsperexperiment} lists the detectors used for each dataset to compute the $F_1$ deterioration. Observe that sometimes only a single detector obtains the greatest $F_1$ score, while sometimes several detectors get the same $F_1$ score.

\paragraph{Q3. False alarms and false negatives.}

\begin{table}[htbp]
\caption{Mean and standard deviation of the false alarm rate (left) and false negative rate (right) obtained by using each method's $\gamma$ estimate to set the threshold (the lower the better). Regarding the false alarms, \ourmethod{} has the third best mean and outperforms \textsc{Qmcd} and \textsc{Karch}, which are the second and third best baseline when measuring the $F_1$ score. On the other hand, \ourmethod{} obtains higher false negative rates than almost all the competitors, due to the fact that the threshold estimators overestimate the true contamination factor.} \label{tab:false_alarms}
\begin{center}
\begin{tabular}{lc}
\multicolumn{2}{c}{\textbf{False Alarm Rate}} \\
\toprule
Method &      Mean $\pm$ std. \\
\midrule
\textsc{Iqr}                 &  $0.009 \pm 0.008$               \\
\textsc{Mtt}                 &  $0.027 \pm  0.024$              \\
\textbf{$\gamma$\textsc{GMM}}&\textbf{0.042}$\pm$\textbf{0.015} \\
\textsc{Qmcd}                &  $0.059 \pm  0.018$              \\
\textsc{Karch}               &  $0.147 \pm  0.047$              \\
\textsc{Chau}                &  $0.190 \pm  0.035$              \\
\textsc{Zscore}              &  $0.221 \pm  0.050$               \\
\textsc{Yj}                  &  $0.390 \pm  0.139$            \\
\textsc{Filter}              &  $0.454 \pm  0.054$        \\
\textsc{Dsn}                 &  $0.477 \pm  0.134$          \\
\textsc{Hist}                &  $0.513 \pm  0.100$         \\
\textsc{Fgd}                 &  $0.533 \pm  0.183$      \\
\textsc{Aucp}                &  $0.591 \pm  0.088$      \\
\textsc{Mcst}                &  $0.611 \pm  0.287$       \\
\textsc{Gesd}                &  $0.616 \pm  0.106$      \\
\textsc{Regr}                &  $0.643 \pm  0.105$      \\
\textsc{Mad}                 &  $0.731 \pm  0.083$       \\
\textsc{Clf}                 &  $0.757 \pm  0.077$      \\
\textsc{Eb}                  &  $0.785 \pm  0.077$       \\
\textsc{Wind}                &  $0.809 \pm  0.076$      \\
 \textsc{Moll}               &  $0.816 \pm  0.082$      \\
 \textsc{Boot}               &  $0.862 \pm  0.079$      \\

\bottomrule
\end{tabular}
\qquad
\begin{tabular}{lc}
\multicolumn{2}{c}{\textbf{False Negative Rate}} \\
\toprule
Method &      Mean $\pm$ std \\
\midrule
 \textsc{Boot} &  $0.001 \pm  0.002$ \\
 \textsc{Wind} &  $0.001 \pm  0.002$ \\
 \textsc{Moll} &  $0.001 \pm  0.002$ \\
   \textsc{Eb} &  $0.001 \pm  0.003$ \\
  \textsc{Mad} &  $0.002 \pm  0.003$ \\
  \textsc{Clf} &  $0.002 \pm  0.003$ \\
 \textsc{Gesd} &  $0.003 \pm  0.005$ \\
 \textsc{Regr} &  $0.003 \pm  0.005$ \\
 \textsc{Aucp} &  $0.004 \pm  0.006$ \\
 \textsc{Hist} &  $0.006 \pm  0.008$ \\
  \textsc{Fgd} &  $0.007 \pm  0.011$ \\
  \textsc{Dsn} &  $0.007 \pm  0.009$ \\
  \textsc{Filter} &  $0.007 \pm  0.009$ \\
 \textsc{Mcst} &  $0.007 \pm  0.012$ \\
   \textsc{Yj} &  $0.009 \pm  0.010$ \\
  \textsc{Zscore} &  $0.017 \pm  0.015$ \\
 \textsc{Chau} &  $0.019 \pm  0.016$ \\
\textsc{Karch} &  $0.021 \pm  0.018$ \\
 \textsc{Qmcd} &  $0.034 \pm  0.024$ \\
\bf{$\gamma$GMM} &  \bf{0.036 $\pm$  0.025} \\
  \textsc{Mtt} &  $0.042 \pm  0.028$ \\
  \textsc{Iqr} &  $0.044 \pm  0.029$ \\
\bottomrule
\end{tabular}

\end{center}
\end{table}

Finally, Table~\ref{tab:false_alarms} shows the false alarm (false positive) rate and the false negative rate. The majority of the threshold estimators provide extremely high estimates for the contamination factor, shown here as extremely low false negative rates, but they would be useless in practice because of their high false alarm rate. In fact, this metric is important as false alarms result in real costs for the company (e.g., turning the wind turbine off to wait until the ice on the blades melts down), while reducing trust in the detection system. Our method reduces the false alarm rate compared to most of the baselines, including \textsc{Qmcd} and \textsc{Karch} that achieve the second and third best $F_1$ scores on average. On the other hand, \textsc{Iqr} and \textsc{Mtt} have the lowest false positive rates, due to the fact that they often underestimate the contamination factor as supported by the false negative table.
